# Supplementary material for: Land Cover Changes Cause Increased Losses during Photosynthetic Extremes
Source: arXiv:2507.18874 source file (2025-08-01)
Supplement: Supplementary file 1 [file figure_sm_regions_wo_trend.tex]

\begin{figure}
 \centering
 \includegraphics[trim = {0.1cm 0.1cm 0.1cm .85cm},clip,width=0.95\columnwidth]{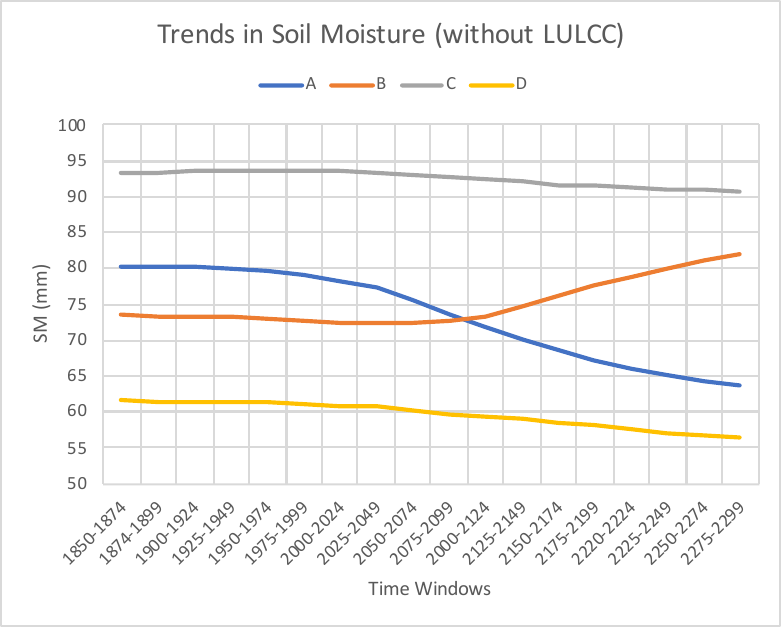}
 \caption{Trends in soil moisture for the simulation without LULCC. The trends are calculated from 1850 as the base year to 25~year increments, as shown in $x$-axis. This figure shows the trends in soil moisture at four randomly selected grid cells (Table~\ref{t:locations_of_regions}) in each region A, B, C, and D.}
\label{f:sm_regions_wo_trend}
\end{figure}
